# Supplementary material for: Injecting linguistic knowledge into BERT for Dialogue State Tracking
Source: arXiv:2311.15623 source file (2024-07-03)
Supplement: Supplementary file 1 [file appendix.tex]

\section{Responsible use of model}
Aside from the limitations mentioned in the main sections, the effect of external injected knowledge on the prediction quality, e.g. whether the knowledge will induce bias in the prediction for downstream tasks, is unknown and should be considered when deploying the model.
The datasets used in this work are checked by the author to be sanitized in terms of personal identifiable information, but whether injecting sensitive data using the proposed method causes information leak in the DST output should be carefully investigated in application.
\section{Implementation details}
\begin{enumerate}
    \item\textbf{Pre-processing} We follow the same procedure in \cite{zhou_automatic_2021} to prepare the datasets for knowledge extraction by CPM, and use the preprocessing utility in Huggingface\footnote{https://huggingface.co/docs/transformers/model\_doc/bert} to prepare the input for BERT.
    \item\textbf{BERT} The BERT model used in all experiments has 12 hidden layers at an embedding width of 768, with 12 attention heads per layer. We used the pre-trained version supplied by HuggingFace\footnote{https://huggingface.co/bert-base-uncased}, governed by Apache 2.0 license permitting research use.
    \item\textbf{Hyperparmeter search} is conducted on a NVIDIA RTX 2080ti for approximately 700 GPU hours. The best found hyperparameter values are recorded in table \ref{hp}.
\end{enumerate}
